# Supplementary material for: Faster Guarantees of Evolutionary Algorithms for Maximization of Monotone Submodular Functions
Source: arXiv:1908.01230 source file (2021-07-05)
Supplement: Supplementary file 1 [file lemmas.tex]

\begin{lemma}
  \label{lemma:chernoffbea}
  The following is Equation \ref{eqn:dsps77th30} of Theorem \ref{theorem:bea}:
  \begin{align}
    P\left(\sum_{i=1}^TY_i < Hk\right) \leq \frac{1}{n}.
  \end{align}
\end{lemma}
\begin{proof}
  Notice that $\ex{\sum_{i=1}^TY_i}=Tp$.
  Therefore
  \begin{align*}
    P\left(\sum_{i=1}^TY_i < H\kappa\right)
    &\overset{a}{\leq} P\left(\sum_{i=1}^TY_i < Tp/2\right) \\
    &\overset{b}{\leq} e^{-Tp/8} \\
    &\overset{c}{\leq} \frac{1}{n}
  \end{align*}
  where (a) is because $T\geq (2e/p)n\ln(1/\epsilon)$;
  (b) is applying Chernoff's bound (Lemma \ref{lemma:chernoff}) with $\eta=1/2$;
  and (c) is because $T\geq 8e/p\ln(n)$.

\end{proof}

\begin{lemma}
  \label{lemma:chernoffeasc}
  The following is Equation \ref{eqn:3dgy} of Theorem \ref{theorem:easc}:
  \begin{align}
    P\left(\sum_{i=1}^TY_i < \min\{n,\ln\left(\frac{1}{\delta}\right)|A^*|\}\right)
    \leq \delta.
  \end{align}
\end{lemma}
\begin{proof}
  Let $\rho$ be the probability of success on any trial
  (the value of $\rho$ is given in Lemma \ref{lemma:success}).
  Then $\ex{\sum_{i=1}^TY_i}=T\rho$.
  Therefore
  \begin{align*}
    P\left(\sum_{i=1}^TY_i < \min\{n, \ln(1/\delta)|A^*|\}\right)
    &\leq P\left(\sum_{i=1}^TY_i < \ln(1/\delta)|A^*|\right) \\
    &\overset{a}{\leq} P\left(\sum_{i=1}^TY_i < T\rho/2\right) \\
    &\overset{b}{\leq} e^{-T\rho/8} \\
    &\overset{c}{\leq} \delta
  \end{align*}
  where (a) is because $T\geq 2en^2\ln(1/\delta)$ combined with the lower bound on $\rho$ given in
  Lemma \ref{lemma:success}; (b) is applying Chernoff's bound (Lemma \ref{lemma:chernoff}) with $\eta=1/2$;
  and (c) is because $T\geq 8en^2\ln(1/\delta)$ combined with the lower bound on $\rho$ given in
  Lemma \ref{lemma:success}.
\end{proof}

\begin{lemma}
  \label{lemma:chernoffbeasc}
  The following is Equation \ref{eqn:dspe30} of Theorem \ref{theorem:beasc}:
  \begin{align}
    P\left(\sum_{i=1}^TY_i < H_q\min\{n,\frac{\ln(1/\delta)|A^*|}{1-\epsilon}\}\right) \leq \delta.
  \end{align}
\end{lemma}
\begin{proof}
  Notice that $\ex{\sum_{i=1}^TY_i}=Tp$.
  Therefore
  \begin{align*}
    P\left(\sum_{i=1}^TY_i< H_q\min\{n,\frac{\ln(1/\delta)|A^*|}{1-\epsilon}\}\right)
    &\leq P\left(\sum_{i=1}^TY_i < H_q\frac{\ln(1/\delta)|A^*|}{1-\epsilon}\right) \\
    &\overset{a}{\leq} P\left(\sum_{i=1}^TY_i < \frac{n\ln(1/\epsilon)\ln(1/\delta)}{\xi(1-\epsilon)}\right) \\
    &\overset{b}{\leq} P\left(\sum_{i=1}^TY_i < \frac{Tp}{2}\right) \\
    &\overset{c}{\leq} e^{-Tp/8} \\
    &\overset{d}{\leq} \delta
  \end{align*}
  where (a) is because by definition $H_q=e\ln(1/\epsilon)/\xi^q$ and using Equation
  \ref{eqn:boundopt}; (b) is because
  $$T\geq 2en\ln(1/\delta)\ln(1/\epsilon)\maxpointer/(\xi p (1-\epsilon))$$;
  (c) is applying Chernoff's bound (Lemma \ref{lemma:chernoff}) with $\eta=1/2$;
  (d) is because $T\geq 8e\ln(n)\maxpointer/p$.
\end{proof}
