# Supplementary material for: Faster Guarantees of Evolutionary Algorithms for Maximization of Monotone Submodular Functions
Source: arXiv:1908.01230 source file (2021-07-05)
Supplement: Supplementary file 2 [file beasc.tex]

As described in Section \ref{section:cover} in the main paper, \bea does not work for
SC because it requires knowledge of $|A^*|$, which is the objective in SC and unknown.
In this section, we discuss the novel algorithm \beascl (\beasc), which is a version of
\bea specifically designed for SC, in greater detail.

\subsubsection{Overview of \beasc}

\begin{algorithm}
   \caption{\beasc$(f, P, T, p, \epsilon, \xi)$: \beascl}
   \label{algorithm:beasc}
   \begin{algorithmic}[1]
     \STATE {\bfseries Input:} \definef; \defineP; \defineT; \definep;
     \defineepsilon; \definexi.
     \STATE {\bfseries Output:} \definepool.
     \STATE $\mathcal S \gets \{ \emptyset \}$
     \STATE $\beta^i\gets 0$, $\ell_i\gets 0$, $H_i \gets e\ln(1/\epsilon)/\xi^i$ \alli
     \FOR {$t\gets 1$ to $T$}
     \STATE $B \gets $ \selectbeasc($\mathcal{S}, p, \beta^i$ \alli )
     \STATE $B' \gets $ \mutate($B$)
     \STATE $\mathcal{S} \gets \add(\mathcal{S}, B', P, f)$
     \IF{$\exists i$ s.t. $|B|=\beta^i$}
     \STATE $\ell_i \gets \ell_i + 1$ \label{line:incellsc}
     \IF{$\ell_i = H_i$}
     \STATE $\ell_i\gets 0$ \label{line:ellsc}
     \IF{$\exists X\in\mathcal{S}$ such that $|X|=\beta^i+1$ and $f(X)\geq f(B)$}
     \STATE $\beta^i\gets \beta^i+1$
     \ENDIF
     \ENDIF
     \ENDIF
     \ENDFOR
     \STATE \textbf{return} $\mathcal{S}$
\end{algorithmic}
\end{algorithm}

\begin{algorithm}
   \caption{\selectbeasc($\mathcal{S},p,\beta^i$ \alli): Selection Algorithm for \beasc}
   \label{algorithm:selectbeasc}
   \begin{algorithmic}[1]
     \STATE {\bfseries Input:} \definepool s.t. \alli $\exists X\in\mathcal{S}$ where $|X|=\beta^i$;
     \definep; $\beta^i\in\{0,...,n\}$ \alli.
     \STATE {\bfseries Output:} \defineB
     \STATE With probability $p$, choose $\beta$ uniformly randomly among
            $\beta^i$ \alli
            and let $B$ be the set in $\mathcal S$ such that $|B|=\beta$;
            otherwise, with probability $(1-p)$, choose uniformly randomly among the
            elements of $\mathcal S$.
     \STATE \textbf{return} $B$
\end{algorithmic}
\end{algorithm}

\beasc is presented in Algorithm \ref{algorithm:beasc}.
\beasc is like \bea, but \selectbeasc (Algorithm \ref{algorithm:selectbeasc})
is biased towards \maxpointersimple many solutions in $\pool$.
\beasc keeps track of variables $\beta^i$ \alli.
With probability $p$, \selectbeasc chooses an $i$ uniformly randomly and then
returns the element in $\pool$ of cardinality $\beta^i$.
Otherwise, \beasc returns an element uniformly randomly from $\pool$.
Initially, $\beta^i=0$ \alli. $\beta^i$ is incremented to $\beta^i+1$ if
(i) there exists as $X\in\pool$ such that
$|X|=\beta^i+1$, and (ii)
on \Hi iterations since the last increment of $\beta^i$ \selectbeasc has chosen
the element in $\pool$ of cardinality $\beta^i$.

\subsubsection{Analysis of \beasc for SC}
The approximation results of \beasc for SC are now presented.
\paragraph{Theorem \ref{theorem:beasc}}
  Suppose we have an instance of SC with optimal solution $A^*$ such that
  $|A^*|\geq 2$.
  Let $P=n$, $\delta\in(0,1]$, \defineepsilon, \definexi, and \beascT
  Then if \ea is run with
  these inputs and $\mathcal{S}$ is its pool at completion,
  $\ex{f(A)} \geq (1-\delta)^2\tau$
  where
  $A=\text{argmax}_{X\in\mathcal{S}, |X|\leq \ln(1/\delta)/(1-\epsilon)|A^*|}f(X).$
%\todo discuss proof

\begin{proof}
  The probability space of all possible runs of \beasc with the stated inputs is considered.
  There exists some fixed $q\in\{1,...,\maxpointer\}$ such that
  \begin{align}
    \xi^qn < |A^*| \leq \xi^{q-1}n. \label{eqn:boundopt}
  \end{align}
  Define $\beta = \beta^q$, where the definition of $\beta^q$ can be found in the pseudocode for
  \beasc (Algorithm \ref{algorithm:beasc}).
  $\omega$ is defined analogously as in the proof of
  Theorem \ref{theorem:bea}:
  \begin{itemize}[noitemsep]
    \item[(i)] Before the first iteration, $\omega=0$.
    \item[(ii)] $\omega$ is incremented at the end of an iteration if
    $\ell_q$ is set to 0 (Line \ref{line:ellsc} of Algorithm \ref{algorithm:beasc}).
  \end{itemize}
  Refer to the proof of Theorem \ref{theorem:bea} for the definitions of
  $\omega_i$, $\beta_i$, and $X_i$.

  The result of Lemma \ref{lemma:expectationbpo} can be shown to hold for the current
  context using the exact same argument with the exception of Equation \ref{eqn:prob}.
  Instead, in order to have the result of Equation \ref{eqn:prob}, one must notice that
  \begin{align*}
    P(\neg F|E) \overset{a}{\leq} \left(1-\frac{|A^*|}{en}\right)^{H_q}
    \overset{b}{\leq} \epsilon
  \end{align*}
  where (a) is using Lemma \ref{lemma:beaprobevent}; and
  (b) is using that $H_q=\ln(1/\epsilon)/\xi^q$ and $n\xi^q<|A^*|$.

  \begin{lemma}
      \label{lemma:successbeasc}
      At the beginning of an iteration of \beasc, the probability
      that $\ell_q$ will be incremented
      during that iteration is
      $p/\left(\maxpointer\right)$.
    \end{lemma}
    \begin{proof}
      This is clear from looking at \selectbeasc.
    \end{proof}

  Let event $F$ be that at the completion of a run of \beasc, $\ell_q$ has been
  incremented $H_q\ln(1/\delta)/(1-\epsilon)|A^*|$
  many times (Line \ref{line:incellsc} of Algorithm \ref{algorithm:beasc}).
  If $\ell_q$ has been incremented $H_q\ln(1/\delta)/(1-\epsilon)|A^*|$
  many times, then one can see that $\omega\geq\min\{n,\ln(1/\delta)/(1-\epsilon)|A^*|\}$.
  %\todo{} Handle $\omega=n$ case.
  Let $A=\text{argmax}_{X\in\mathcal{S}, |X|\leq\ln(1/\delta)/(1-\epsilon)|A^*|}f(X)$. Then
  \begin{align}
    \ex{f(A)|F} &\overset{a}{\geq}
    \left(1-\left(1-\frac{1-\epsilon}{|A^*|}\right)^{\ln(1/\delta)/(1-\epsilon)|A^*|}\right)f(A^*) \nonumber \\
    &\geq (1-\delta)\tau. \label{eqn:ksj3422}
  \end{align}
  where (a) is by an analogous argument to that used in Theorem \ref{theorem:ea} but
  instead using Lemma \ref{lemma:expectationbpo}.

  We now apply Chernoff's Bound in order to bound the probability of event
  $F$ not occurring.
  Again, a run of \beasc is considered as a
  series of independent Bernoulli trials: Each
  iteration is a trial and it is a success if $\ell_q$ is incremented. Let the random variable
  associated with iteration $i$ be $Y_i$.
  Then Chernoff's bound (Lemma \ref{lemma:chernoff}) as well as the fact that
  \beascT, can be used to show that
  \begin{align}
    P\left(\sum_{i=1}^TY_i < H_q\frac{\ln(1/\delta)|A^*|}{1-\epsilon}\right) \leq \delta. \label{eqn:dspe30}
  \end{align}
  where details are given in Lemma \ref{lemma:chernoffbeasc}.
  Finally, the Law of Total Probability along with Equations \ref{eqn:ksj3422} and \ref{eqn:dspe30}.
  gives the result stated in Theorem \ref{theorem:beasc}.
\end{proof}
