# Supplementary material for: Faster Guarantees of Evolutionary Algorithms for Maximization of Monotone Submodular Functions
Source: arXiv:1908.01230 source file (2021-07-05)
Supplement: Supplementary file 3 [file cover.tex]

Our results for SC were briefly described in Section \ref{section:cover} in the main
paper. The theoretical contributions of the paper for SC are presented in more detail in this section.
In particular, a new theoretical analysis of the algorithm \ea is presented for
SC in Section \ref{appendix:easc}, and
the novel algorithm \beascl (\beasc), which is a version of \bea for SC,
is presented and analyzed for SC in Section \ref{appendix:beasc}.

\subsubsection{appendix:easc}

\beal (\bea) is a novel evolutionary algorithm with nearly the same approximation
results as \ea for SM, but in this section it is proven that
\bea finds a \bearatio approximate solution in expectation in \beatimenop time.
Despite \bea being faster than \ea by a factor of \budget, \bea is only different
from \ea in that its selection procedure is biased instead of choosing uniformly
randomly.

\beascl (\beasc) is a version of \bea for SC that does not require knowledge of $|A^*|$.
It is proven in Section \ref{section:beascanalysis} that \beasc finds approximate solutions that are
near feasible in expectation for SC in \beasctime time.
To the best of our knowledge, there does not yet exist an \sg analogue proposed for
SC, and thus \beasc is the first \beasctime time algorithm analyzed for SC.
\beasc is like \bea, but is biased towards \maxpointersimple many solutions in
its pool, each corresponding to an estimate of $|A^*|$.
The algorithm \beasc is described in Section \ref{section:beascoverview} and pseudocode
for \beasc is provided in Section \ref{appendix:beasc} in the appendix.

\subsubsection{Overview of \beasc}
\label{section:beascoverview}
\beasc (Algorithm \ref{algorithm:beasc} in Section \ref{appendix:beasc} in the appendix)
is similar to \bea, and therefore only the differences between \beasc and \bea
are described here.
In addition to the parameters of \bea, \beasc requires the parameter \definexi.
\beasc keeps track of variables $\beta^i$ \alli.
\selectbeasc returns an element of $\pool$ of cardinality $\beta^i$, where $i$ is chosen
uniformly randomly (there always exists one), with probability $p$,
and otherwise chooses uniformly randomly from $\pool$.
Initially, $\beta^i=0$ \alli.
$\beta^i$ is incremented when the following conditions have been met on \Hi many times:
\selectbeasc results in the selection of the element in $\pool$ is cardinality
$\beta^i$, and \mutate resulted in the flipped membership of a
single element.
The details of \beasc, as well as the subroutine \selectbeasc
can be found in Algorithm \ref{algorithm:beasc} of Section \ref{appendix:beasc} in the appendix.
It should be noted that \beasc is not equivalent to running a separate \bea with $\beta=\beta^i$ for
each $i$, because there is one pool $\pool$ that is being shared.

\subsubsection{Analysis of \beasc for SC}
\label{section:beascanalysis}
The approximation results of \beasc for SC are now presented.
In contrast to Theorem \ref{theorem:bea}, it is the feasibility that is in expectation.
\begin{theorem}
  \label{theorem:beasc}
  Suppose we have an instance of SC with optimal solution $A^*$ such that
  $|A^*|\geq 2$.
  Let $P=n$, $\delta\in(0,1]$, \defineepsilon, \definexi, and \beascT
  Then if \ea is run with
  these inputs and $\mathcal{S}$ is its pool at completion,
  $\ex{f(A)} \geq (1-1/n)(1-\delta)\tau$
  where
  $A=\text{argmax}_{X\in\mathcal{S}, |X|\leq \ln(1/\delta)/(1-\epsilon)|A^*|}f(X).$
\end{theorem}
Recall that in \bea in Section \ref{section:bea} that $\beta$ is advanced if $\ell$ has been
incremented $n/\kappa\ln(1/\epsilon)$ many times.
A difficulty with applying \bea to SC is that the cardinality of the optimal solution
(\budget in SM) is unknown.
This difficulty is ameliorated in \beasc by making $\maxpointer$ guesses for $|A^*|$,
each with a corresponding $\beta_i$. The $\beta_i$ corresponding to the closest
lower bound of $|A^*|$ is chosen with probability $p/\maxpointer$, resulting in a
$\maxpointer$ slow down compared to \bea.

\begin{proof}
  The probability space of all possible runs of \beasc with the stated inputs is considered.
  There exists some fixed $q\in\{1,...,\maxpointer\}$ such that
  \begin{align}
    \xi^qn < |A^*| \leq \xi^{q-1}n. \label{eqn:boundopt}
  \end{align}
  Define $\beta = \beta^q$, where the definition of $\beta^q$ can be found in the pseudocode for
  \beasc (Algorithm \ref{algorithm:beasc}).
  $\omega$ is defined analogously as in the proof of
  Theorem \ref{theorem:bea}:
  \begin{itemize}[noitemsep]
    \item[(i)] Before the first iteration, $\omega=0$.
    \item[(ii)] $\omega$ is incremented at the end of an iteration if
    $\ell_q$ is set to 0 (Line \ref{line:ellsc} of Algorithm \ref{algorithm:beasc}).
  \end{itemize}
  Refer to the proof of Theorem \ref{theorem:bea} for the definitions of
  $\omega_i$, $\beta_i$, and $X_i$.

  The result of Lemma \ref{lemma:expectationbpo} can be shown to hold for the current
  context using the exact same argument with the exception of Equation \ref{eqn:prob}.
  Instead, in order to have the result of Equation \ref{eqn:prob}, one must notice that
  \begin{align*}
    P(\neg F|E) \overset{a}{\leq} \left(1-\frac{|A^*|}{en}\right)^{H_q}
    \overset{b}{\leq} \epsilon
  \end{align*}
  where (a) is using Lemma \ref{lemma:beaprobevent}; and
  (b) is using that $H_q=\ln(1/\epsilon)/\xi^q$ and $n\xi^q<|A^*|$.

  \begin{lemma}
      \label{lemma:successbeasc}
      At the beginning of an iteration of \beasc, the probability
      that $\ell_q$ will be incremented
      during that iteration is
      $p/\left(\maxpointer\right)$.
    \end{lemma}
    \begin{proof}
      This is clear from looking at \selectbeasc.
    \end{proof}

  Let event $F$ be that at the completion of a run of \beasc, $\ell_q$ has been
  incremented $H_q\ln(1/\delta)/(1-\epsilon)|A^*|$
  many times (Line \ref{line:incellsc} of Algorithm \ref{algorithm:beasc}).
  If $\ell_q$ has been incremented $H_q\ln(1/\delta)/(1-\epsilon)|A^*|$
  many times, then one can see that $\omega\geq\min\{n,\ln(1/\delta)/(1-\epsilon)|A^*|\}$.
  %\todo{} Handle $\omega=n$ case.
  Let $A=\text{argmax}_{X\in\mathcal{S}, |X|\leq\ln(1/\delta)/(1-\epsilon)|A^*|}f(X)$. Then
  \begin{align}
    \ex{f(A)|F} &\overset{a}{\geq}
    \left(1-\left(1-\frac{1-\epsilon}{|A^*|}\right)^{\ln(1/\delta)/(1-\epsilon)|A^*|}\right)f(A^*) \nonumber \\
    &\geq (1-\delta)\tau. \label{eqn:ksj3422}
  \end{align}
  where (a) is by an analogous argument to that used in Theorem \ref{theorem:ea} but
  instead using Lemma \ref{lemma:expectationbpo}.

  We now apply Chernoff's Bound in order to bound the probability of event
  $F$ not occurring.
  Again, a run of \beasc is considered as a
  series of independent Bernoulli trials: Each
  iteration is a trial and it is a success if $\ell_q$ is incremented. Let the random variable
  associated with iteration $i$ be $Y_i$.
  Then Chernoff's bound (Lemma \ref{lemma:chernoff}) as well as the fact that
  \beascT, can be used to show that
  \begin{align}
    P\left(\sum_{i=1}^TY_i < H_q\frac{\ln(1/\delta)|A^*|}{1-\epsilon}\right) \leq \delta. \label{eqn:dspe30}
  \end{align}
  where details are given in Lemma \ref{lemma:chernoffbeasc}.
  Finally, the Law of Total Probability along with Equations \ref{eqn:ksj3422} and \ref{eqn:dspe30}.
  gives the result stated in Theorem \ref{theorem:beasc}.
\end{proof}
