# Supplementary material for: Faster Guarantees of Evolutionary Algorithms for Maximization of Monotone Submodular Functions
Source: arXiv:1908.01230 source file (2021-07-05)
Supplement: Supplementary file 4 [file easc.tex]

Our results on \ea for SC are briefly described in Section \ref{section:cover} in the main
paper. In this sections, further discussion and a proof of Theorem \ref{theorem:easc}
is provided.
To the best of our knowledge, \ea has not previously been shown to produce an approximate
solution for SC in expected polynomial time. Therefore Theorem \ref{theorem:easc},
which states that \ea finds a solution with a constant factor approximation that is near feasible
in expectation in time $\mathcal{O}(n^2\ln(n))$, is the first such result. \ea has been analyzed for a more general
problem than SC \qiansc, but whether the solution is expected in polynomial time depends
on the particular instance. It is possible to adjust the argument of \qiansct in order to
show that an approximate solution for SC is expected in time \qiansctime, however by
using a different argument and instead having near feasibility in expectation
we are able to remove a factor of $n/\ln(n)$ from this runtime in Theorem \ref{theorem:easc}.
%\todo Fix runtime for SC.

\paragraph{Theorem \ref{theorem:easc}}
  Suppose we have an instance of SC with optimal solution $A^*$.
  Let $P=n$, $\delta\in(0,1]$,
  and \eascT.
  Then if \ea is run with
  these inputs and $\mathcal{S}$ is its pool at completion,
  $\ex{f(A)} \geq (1-\delta)^2\tau$
  where
  $A=\text{argmax}_{X\in\mathcal{S}, |X|\leq \ln(1/\delta)|A^*|}f(X).$

%\todo Discuss proof, how we can't find the solution.

\begin{theorem}
  \label{theorem:easc}
  Suppose we run \ea with input monotone submodular \definef
  and $P=n+1$.
  Then for any $\tau \leq f(U)$ and \definedelta
  if \poolb is the pool of \ea at the end of iteration
  \eascT of the for loop of \ea then
  $$\ex{\max_{X\in\mathcal{S}, |X|\leq \ln(1/\delta)|A^*|}f(X)}
   \geq (1-1/n)(1-\delta)\tau.$$
\end{theorem}

\begin{proof}
  Consider any $\tau\leq f(U)$. Define $A^*=\argmin_{f(X)\geq\tau}|X|$.
  $\omega$ and $\beta$ are defined in the same way as in the proof of Theorem
  \ref{theorem:ea}.
  Then Lemmas \ref{lemma:expectation}, \ref{lemma:replace}, and \ref{lemma:bernoulli}
  in the proof of Theorem \ref{theorem:ea} also hold in this context.
  The proof of Theorem \ref{theorem:easc} proceeds in the same manner as the proof of
  Theorem \ref{theorem:ea}, except we analyze the event that $\omega$ reaches
  $\ln(1/\delta)|A^*|$ instead of $|A^*|.$

  Let event $F$ be that at the completion of a run of \ea, $\omega\geq\ln(1/\delta)|A^*|$.
  Then it clearly follows from Lemmas \ref{lemma:expectation} and \ref{lemma:replace}
  that
  \begin{align}
    \ex{\max_{X\in\mathcal{S}, |X|\leq \ln(1/\delta)|A^*|}f(X)}
    \geq (1-1/n)(1-\delta)\tau. \label{eqn:ksj2}
  \end{align}
  Then the probability of event $F$ not occurring after
  \eascT
  iterations of \bea can be bounded
  by $1/n$ using the Chernoff bound, and then the law of total
  probability applied.
  The details of the argument can be found in Section \ref{appendix:bealemmas}.

%  $\omega\geq \min\{n,\ln(1/\delta)|A^*|\}$.
%  Define $$A=\text{argmax}_{X\in\mathcal{S}, |X|\leq\ln(1/\delta)|A^*|}f(X).$$
%  Then by a similar argument to that used to prove Equation \ref{eqn:hfd66672} of
%  Theorem \ref{theorem:ea}, it can be shown that
%  \begin{align}
%    \ex{f(A)|F} &\geq \ex{f(X_t)|F} \nonumber \\
%    &\geq (1-\delta)\tau. \label{eqn:ksj2}
%  \end{align}
%  In addition, as in the proof of Theorem \ref{theorem:ea}, a run of \ea is considered as a
%  series of independent Bernoulli trials: Each
%  iteration is a trial and it is a success if $\omega$ is incremented. Let the random variable
%  associated with iteration $i$ be $Y_i$, hence $Y_i=1$ if $\omega$ is incremented at iteration $i$
%  and $Y_i=0$ otherwise.
%  Then Chernoff's bound (Lemma \ref{lemma:chernoff}) as well as the fact that
%  $T\geq\max\{2en^2\ln(1/\delta), 8en^2\ln(1/\delta)\}$, can be used to show that
%  \begin{align}
%    P\left(\sum_{i=1}^TY_i < \min\{n,\ln\left(\frac{1}{\delta}\right)|A^*|\}\right)
%    \leq \delta. \label{eqn:3dgy}
%  \end{align}
%  where the details may be found in Lemma \ref{lemma:chernoffeasc}.
%  Finally, Equations \ref{eqn:ksj2} and \ref{eqn:3dgy} along with the Law of Total
%  Probability prove the result of Theorem \ref{theorem:easc}.
\end{proof}
