# Supplementary material for: Faster Guarantees of Evolutionary Algorithms for Maximization of Monotone Submodular Functions
Source: arXiv:1908.01230 source file (2021-07-05)
Supplement: Supplementary file 5 [file weaksubmodular.tex]

Recently, attention has also been paid to applications
that require the maximization of a monotone function
that is only \textit{approximately} submodular in some sense. Examples of such applications include
dictionary selection \citep{Das2011,cevher2011greedy}, data summarization \citep{chen2017weakly},
viral marketing \citep{Kuhnle2018a,pmlr-v97-crawford19a},
and statistical learning theory \citep{Elenberg2018}.
An important class of approximately submodular functions is that of $\gamma$-weakly
submodular functions
\citep{Das2011}, where $\gamma\in[0,1]$ measures how
close to submodular a function.
A function $f:2^U\to\mathbb{R}_{\geq 0}$ defined on subsets of a ground set $U$ of
size $n$ is \emph{$\gamma$-weakly submodular} if for all
$X\subseteq Y \subseteq U$, and $u\notin Y$,
$\sum_{u\in Y\setminus X}\Delta f(X,u) \geq \gamma \Delta f(X,Y)$.
If $\gamma = 1$, then $f$ is \emph{submodular}.

The alternative optimization problem that is SM but instead $f$ is
assumed to be monotone $\gamma$-weakly submodular is called $\gamma$-weakly submodular
maximization ($\gamma$-WSM).
The results presented in this paper readily extend to $\gamma$-WSM, but with different
approximation guarantees that depend on $\gamma$.
First, an
alternative version of Lemma \ref{lemma:gain} that is needed for the alternative
analyses is provided.

\paragraph{Lemma \ref{lemma:gain} (\wsm)}
  Let $B,X\subseteq U$, $X\neq\emptyset$.
  Suppose that $B$ is input to \mutate, and consider the probability space of
  all possible outputs of \mutate. Let $E$ be the event that \mutate returns
  $B\cup\{x\}$ for some $x\in X\setminus B$ or $B\setminus\{x\}$ for some $x\in X\cap B$. Then
  \begin{align*}
    \ex{\delt{B}{x}|E} \geq \frac{\gamma}{|X|}(f(X)-f(B)).
  \end{align*}
\begin{proof}
  Similar to the original proof of Lemma \ref{lemma:gain}, it is the case that
  \begin{align*}
    \ex{\delt{B}{x}|E} &= \frac{1}{|X|}\sum_{y\in X}\delt{B}{y} \\
                       &\overset{a}{\geq} \frac{\gamma}{|X|}(f(X)-f(B))
  \end{align*}
  where (a) follows from the monotonicity and $\gamma$-weak submodularity of $f$.
\end{proof}

Alternative statements of Theorems
\ref{theorem:ea} and \ref{theorem:bea}
for monotone $\gamma$-weakly submodular functions are provided.

\paragraph{Theorem \ref{theorem:ea} ($\gamma$-weakly submodular)}
  Suppose we have an instance of $\gamma$-WSM
  with optimal solution $A^*$. Let
  $P=2 \kappa$,
  and $T\geq\max\{4en\kappa,16en\ln(n)\}$. Then if \ea is run with
  these inputs and $\mathcal{S}$ is its pool at completion,
  $\ex{f(A)} \geq (1-1/n)(1-1/e^{\gamma})f(A^*),$
  where
  $A=\text{argmax}_{X\in\mathcal{S}, |X|\leq \kappa}f(X).$
\begin{proof}
  The proof is the same as Theorem \ref{theorem:ea} except use the alternative
  version of Lemma \ref{lemma:gain} provided above starting at Equation \ref{eqn:xssda3}.
\end{proof}

\paragraph{Theorem \ref{theorem:bea} ($\gamma$-weakly submodular)}
  Suppose we have an instance of \wsm with optimal solution $A^*$. Let
  $P=2 \kappa$, $p\in(0,1]$,
  $H=(n/k)\ln(1/\epsilon)$ for $\epsilon > 0$, and \beaT.
  Then if \bea is run with
  these inputs and $\mathcal{S}$ is its pool at completion,
  $\ex{f(A)} \geq (1-1/n)(1-1/e^{\gamma}-\epsilon)f(A^*),$
  where
  $A=\text{argmax}_{X\in\mathcal{S}, |X|\leq \kappa}f(X).$
\begin{proof}
  The proof is the same as Theorem \ref{theorem:bea} except use the alternative
  version of Lemma \ref{lemma:gain} provided above starting at Equations
  \ref{eqn:3} and \ref{eqn:4}.
\end{proof}

%\paragraph{Theorem \ref{theorem:easc} (\wsm)}
%  Suppose we have an instance of \wsm with optimal solution $A^*$.
%  Let $P=n$, $\delta\in(0,1]$,
%  and \eascT.
%  Then if \ea is run with
%  these inputs and $\mathcal{S}$ is its pool at completion,
%  $\ex{f(A)} \geq (1-1/n)(1-\delta)\tau$
%  where
%  $A=\text{argmax}_{X\in\mathcal{S}, |X|\leq \ln(1/\delta)/\gamma|A^*|}f(X).$
%\begin{proof}
%  \todo
%\end{proof}

%\paragraph{Theorem \ref{theorem:beasc} (\wsm)}
%  Suppose we have an instance of SC with optimal solution $A^*$ such that
%  $|A^*|\geq 2$.
%  Let $P=n$, $\delta\in(0,1]$, \defineepsilon, \definexi, and \beascT
%  Then if \beasc is run with
%  these inputs and $\mathcal{S}$ is its pool at completion,
%  $\ex{f(A)} \geq (1-1/n)(1-\delta)\tau$
%  where
%  $A=\text{argmax}_{X\in\mathcal{S}, |X|\leq \ln(1/\delta)/(\gamma(1-\epsilon))|A^*|}f(X).$
%\begin{proof}
%  \todo
%\end{proof}

%
