# Supplementary material for: Faster Guarantees of Evolutionary Algorithms for Maximization of Monotone Submodular Functions
Source: arXiv:1908.01230 source file (2021-07-05)
Supplement: Supplementary file 6 [file beascpseudocode.tex]

\begin{algorithm}
   \caption{\beasc$(f, P, T, p, \epsilon, \xi)$: \beascl}
   \label{algorithm:beasc}
   \begin{algorithmic}[1]
     \STATE {\bfseries Input:} \definef; \defineP; \defineT; \definep;
     \defineepsilon; \definexi.
     \STATE {\bfseries Output:} \definepool.
     \STATE $\mathcal S \gets \{ \emptyset \}$
     \STATE $\beta^i\gets 0$, $\ell_i\gets 0$, $H_i \gets e\ln(1/\epsilon)/\xi^i$ \alli
     \FOR {$t\gets 1$ to $T$}
     \STATE $B \gets $ \selectbeasc($\mathcal{S}, p, \beta^i$ \alli )
     \STATE $B' \gets $ \mutate($B$)
     \STATE $\mathcal{S} \gets \add(\mathcal{S}, B', P, f)$
     \IF{$\exists i$ s.t. $|B|=\beta^i$}
     \STATE $\ell_i \gets \ell_i + 1$ \label{line:incellsc}
     \IF{$\ell_i = H_i$}
     \STATE $\ell_i\gets 0$ \label{line:ellsc}
     \IF{$\exists X\in\mathcal{S}$ such that $|X|=\beta^i+1$ and $f(X)\geq f(B)$}
     \STATE $\beta^i\gets \beta^i+1$
     \ENDIF
     \ENDIF
     \ENDIF
     \ENDFOR
     \STATE \textbf{return} $\mathcal{S}$
\end{algorithmic}
\end{algorithm}

\begin{algorithm}
   \caption{\selectbeasc($\mathcal{S},p,\beta^i$ \alli): Selection Algorithm for \beasc}
   \label{algorithm:selectbeasc}
   \begin{algorithmic}[1]
     \STATE {\bfseries Input:} \definepool s.t. \alli $\exists X\in\mathcal{S}$ where $|X|=\beta^i$;
     \definep; $\beta^i\in\{0,...,n\}$ \alli.
     \STATE {\bfseries Output:} \defineB
     \STATE With probability $p$, choose $\beta$ uniformly randomly among
            $\beta^i$ \alli
            and let $B$ be the set in $\mathcal S$ such that $|B|=\beta$;
            otherwise, with probability $(1-p)$, choose uniformly randomly among the
            elements of $\mathcal S$.
     \STATE \textbf{return} $B$
\end{algorithmic}
\end{algorithm}
